# Supplementary material for: Topics in Deep Learning and Optimization Algorithms for IoT Applications in Smart Transportation
Source: arXiv:2210.07246 source file (2022-10-13)
Supplement: Supplementary file 1 [file appendix.tex]

Appendix goes here...
